# Supplementary material for: Early stages of polycrystalline diamond deposition: Laser reflectance at substrates with growing nanodiamonds
Source: arXiv:2210.00776 ancillary file (2022-10-03)
Supplement: Supplementary file 1 [file SupportingInformation.pdf]

Supporting information

Early stages of polycrystalline diamond deposition: Laser  
reflectance at substrates with growing nanodiamonds

David Vázquez-Cortés, Stoffel D. Janssens,  
Burhannudin Sutisna and Eliot Fried<sup>†</sup>

Mathematics, Mechanics, and Materials Unit (MMMU), Okinawa Institute of Science and Technology  
Graduate University (OIST), 1919-1 Tancha, Onna-son, Kunigami-gun, Okinawa, Japan 904-0495

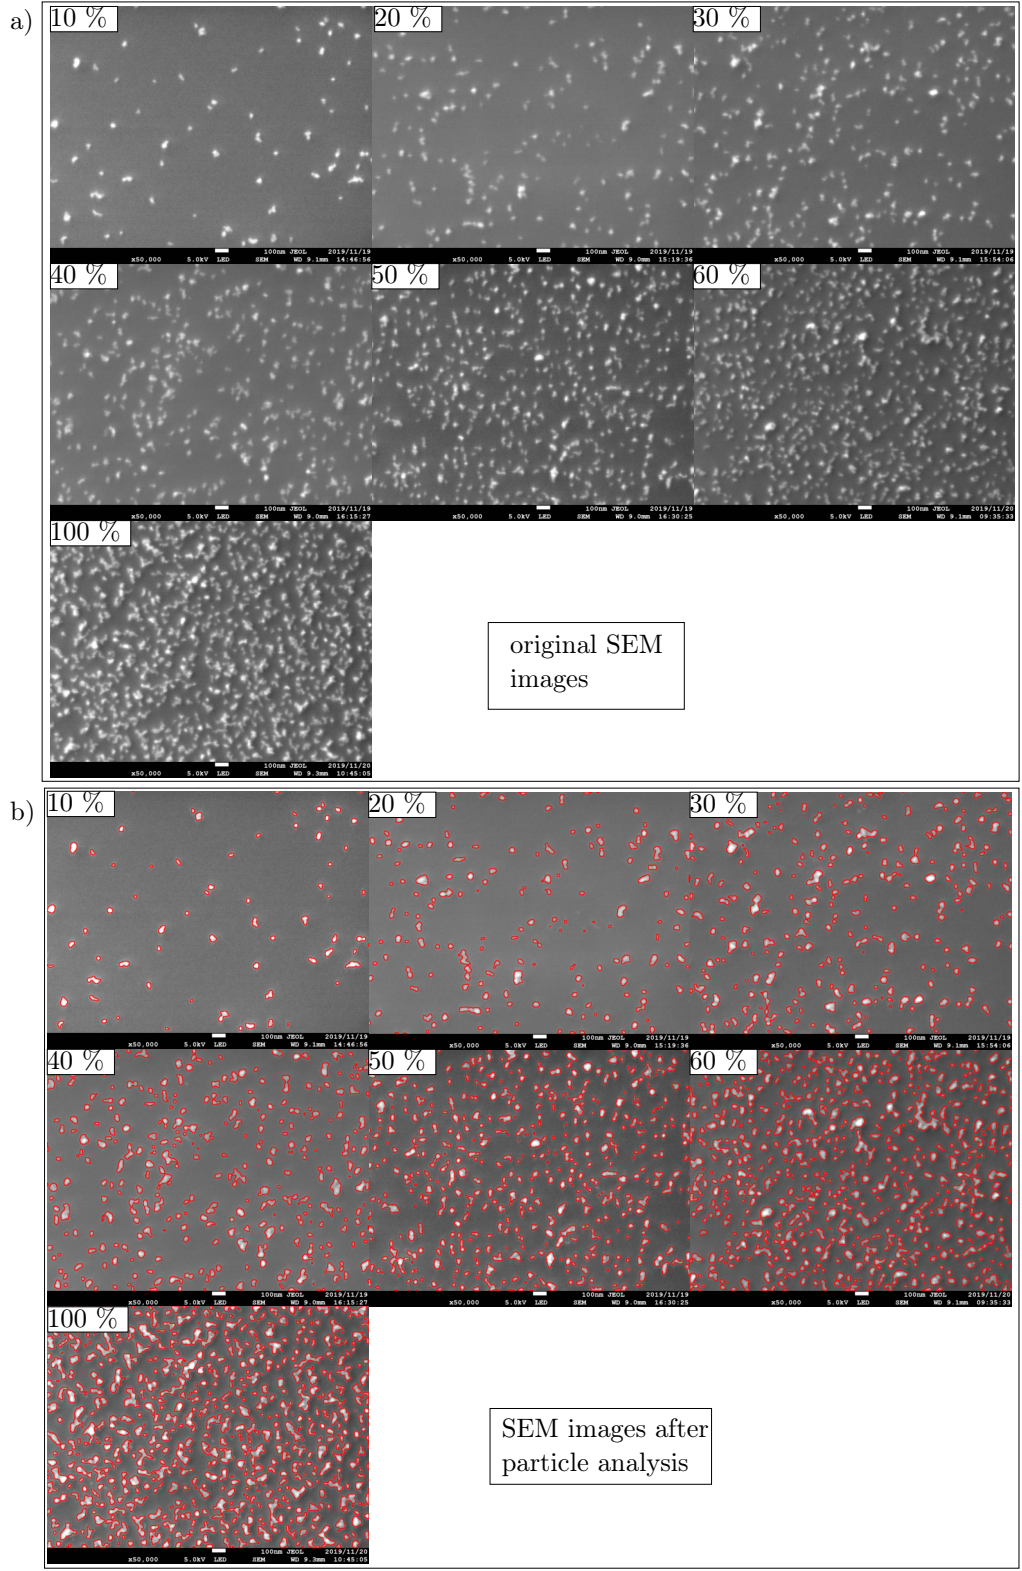

Figure S1: Full set of SEM images from the samples substrates after seeding with varying nanodiamond suspension concentration, before (a) and after (b) analysis by our homemade python script. The python script surrounds by a red contour each particle detected. The red contours are used to assess the accuracy of the script to detect the diamond grains by visual observation of not surrounded contours or contours where no diamond grain is visible.

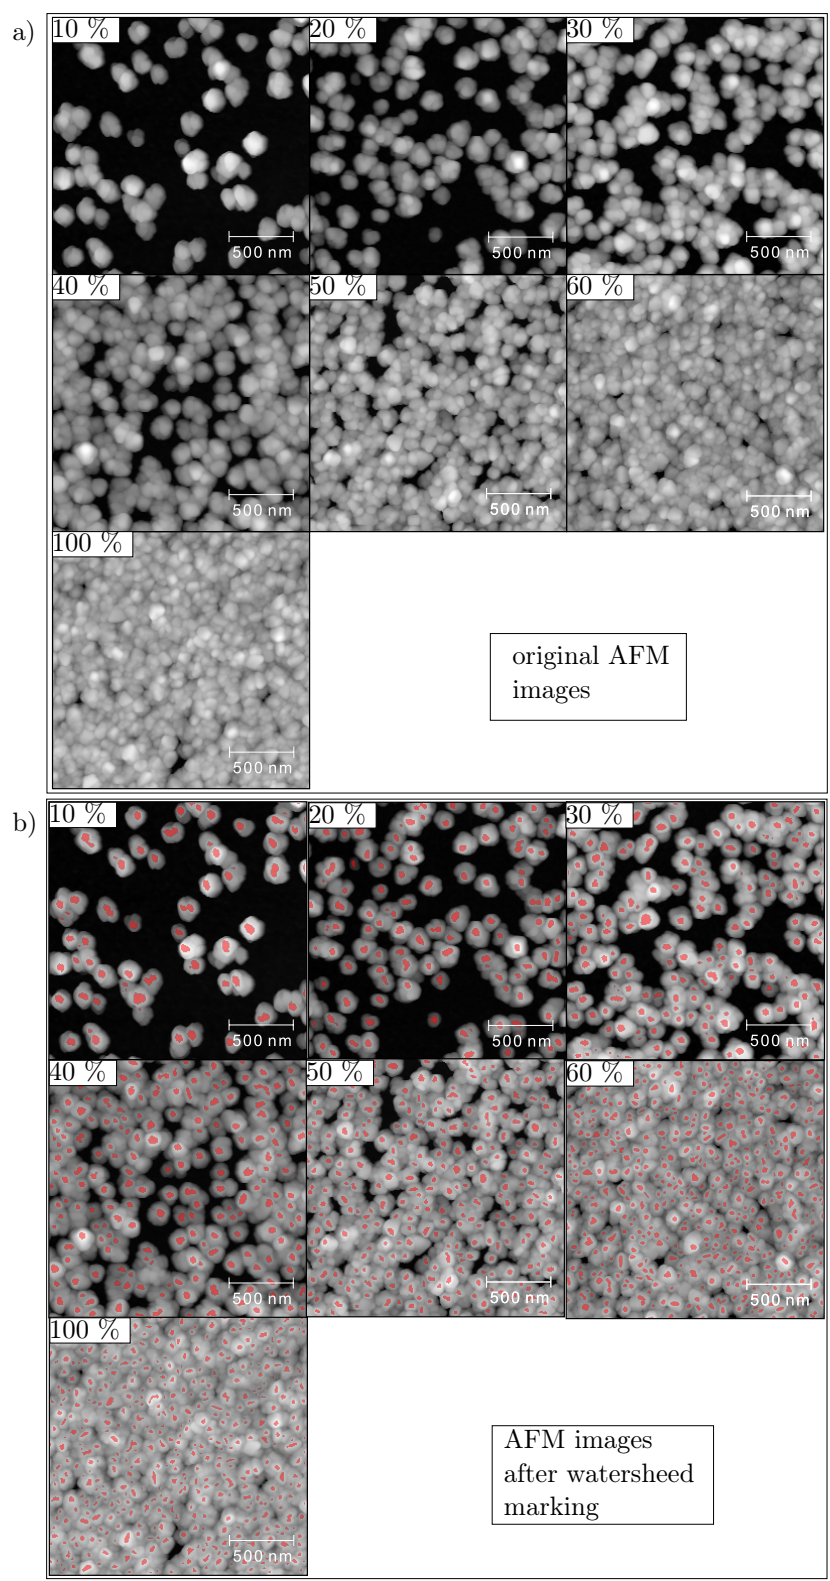

Figure S2: Full set of AFM images from samples seeded with varying nanodiamond suspension concentrations after diamond growth, before and after grain marking with the "watersheed" method available in Gwyddion software.

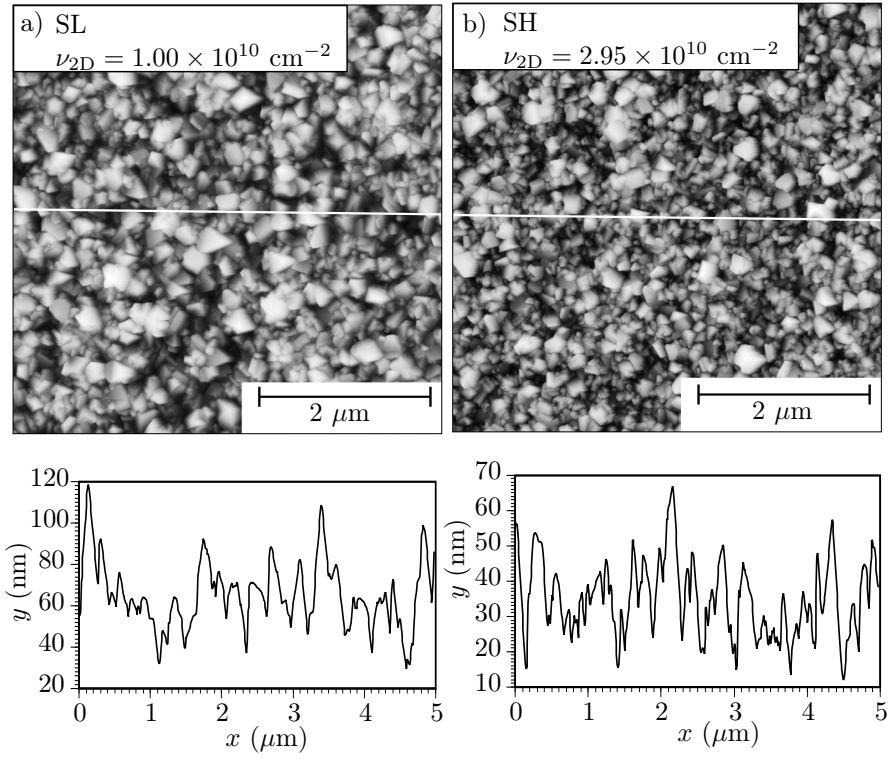

Figure S3:  $5 \times 5 \mu\text{m}^2$  AFM images from the surface of polycrystalline diamond films grown on substrates seeded with low  $\nu_{2D} = 1.00 \times 10^{10} \text{ cm}^{-2}$  (SL) and high  $\nu_{2D} = 2.95 \times 10^{10} \text{ cm}^{-2}$  (SH) seed densities. Height profiles along the selected white lines on the AFM images are also included. The growth time and growth rate were set to 5 hours and 36 nm/hour for a total thickness of  $\approx 180$  nm.
